# Supplementary material for: Muon-spin-rotation study of the magnetic structure in the tetragonal antiferromagnetic state of weakly underdoped Ba$ _{1-x} $K$ _{x} $Fe$ _{2} $As$ _{2} $
Source: arXiv:1506.00786 ancillary file (2015-09-14)
Supplement: Supplementary file 1 [file Mallett_BKFA_muSR_tAFphase_SOM_v2.pdf]

# Supplementary Online Material: Muon-spin-rotation study of the magnetic structure in the tetragonal antiferromagnetic state of weakly underdoped $Ba_{1-x}K_xFe_2As_2$

B.P.P. Mallett[1], Yu. G. Pashkevich[2], A. Gusev[2], Th. Wolf[3], and C. Bernhard[1]

[1] *University of Fribourg, Department of Physics and Fribourg Center for Nanomaterials, Chemin du Muse 3, CH-1700 Fribourg, Switzerland.*

[2] *O. O. Galkin Donetsk Institute for Physics and Engineering NAS of Ukraine, 03680 Kyiv, Ukraine.*

[3] *Institute of Solid State Physics, Karlsruhe Institute of Technology, Postfach 3640, Karlsruhe 76021, Germany.*

## Muon site calculation

The space group symmetry of $Ba_{1-x}K_xFe_2As_2$ (BKFA) in the paramagnetic phase is I4/mmm with one formula unit (Z=1) in the primitive cell. The Ba ions reside in the 1a – position (0,0,0), As in the 2e – position (0,0,$z_{As}$) and Fe in the 2d – position (0,1/2,1/4). Note that the crystallographic unit cell differs from the primitive cell which is built by primitive translations: $a_1$=(-a/2;b/2;c/2)=(-τ;τ;$τ_c$), $a_2$=(a/2;-b/2;c/2)=(τ;-τ;$τ_c$); $a_3$=(a/2;b/2,-c/2) =(τ;τ;-$τ_c$). We analyzed the position of the muon stopping sites for a K content of x=0.2465 with the structural room temperature data: a=b=3.9343 Å, c=13.2061 Å, and $z_{As}$ = 0.35408 Å.

We used a modified Thomas Fermi approach [S1] that allows a direct determination of the self-consistent distribution of the valence electron density from which the electrostatic potential can be restored. The local, interstitial minima of this electrostatic potential are identified as muon stopping sites.

For the same purposes we performed more elaborated *ab initio* calculations within the framework of density functional theory (DFT). We applied the all-electron full-potential linearized augmented plane wave method (Elk code) [S2] with the local spin density approximation [S3] for the exchange correlation potential and with the revised generalized gradient approximation of Perdew-Burke-Ernzerhof [S4]. The calculations were performed on a 9x9x6 grid which corresponds to 60 points in the irreducible Brillouin zone. In both approaches we used a supercell 2a x 2b x c and supposed x=0.25 (e.g. $Ba_{0.75}$ $K_{0.25}$ $Fe_2As_2$). This allows one to explicitly incorporate K ions which were positioned in the supercell at coordinates K(1) - (a, b, 0) and K(2) - (3/2a, 3/2b, 1/2c).

The DFT and modified Thomas Fermi approaches give almost the same answers. We observed three possible types of muon sites. Two of them are located on the line along the c-direction connecting the nearest Ba or K and As ions at the coordinates (0, 0, $z_\mu$) with $z_\mu$ = 0.191 for Ba and $z_\mu$ = 0.170 for K. In the I4/mmm setting these muon sites have a 2e – local point symmetry (4mm), i.e. the same as the As ions. We have verified that the dipolar fields from a given magnetic structure of the Fe moments have nearly the same magnitudes at these two positions. Accordingly, in the dipolar field calculations we discuss only one type of muon stopping site.

The third muon site is located in the Ba *ab*-plane close to the line connecting the As-As ions along the *c*-direction. In the I4/mmm setting it has a rather high 4j – local point symmetry (m2m) at the coordinates (0.4, 0.5, 0). Its electrostatic potential is roughly 20% less than the potential of the previous two sites. Accordingly, this site should be partially populated in the

μSR experiment. The probability of the occupation of this secondary site, as compared to the one of the majority site, we calculate to be 0.24 which agrees rather well with the experimental amplitude ratio of $A_2^{os}/A_1^{os} \approx 0.2$ (see Fig. 2 of the paper). The qualitative changes of the local dipole fields on this minority site at the o-AF to t-AF transition are very similar to the ones on the majority muon sites. Accordingly, in the following and in the paper we do not further discuss this minority muon site and focus instead on the changes of the local dipole field on the majority muon site.

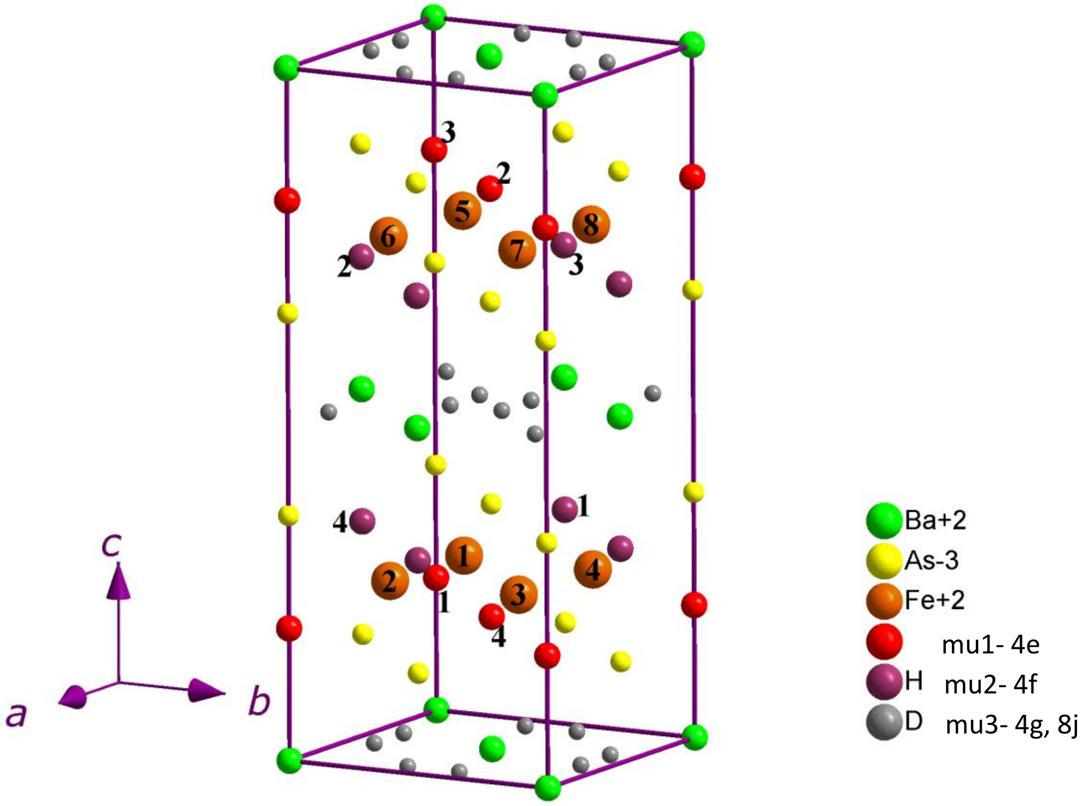


***Figure S1**: Sketch of the unit cell of $Ba_{1-x}K_xFe_2As_2$ in the tetragonal subgroup P4/mbm of the space group I4/mmm. Atoms and muon stopping sites are in the positions; Ba1 - 2a (0,0,0), Ba2 – 2c (0,1/2,1/2), As1/$\mu$1 – 4e (0,0,$z_1$(As/$\mu$)) with $z_1$(As)=$z_1$($\mu$)=1/2, As2/$\mu$2 – 4f (0,1/2, $z_2$(As/$\mu$)) with $z_2$(As)=0.35408 and $z_2$($\mu$)=0.188, Fe – 8k (x, x+1/2, z) with x=1/4, z=1/4, $\mu$3 - 4g (0.4, 0.9 ,0) and 4g – (0.1, 0.6, 0) and 8j – (0.1, 0.1, 0.5). The enumeration of the Fe- and $\mu$1 and $\mu$2 sites is indicated.*

## Calculations of the dipolar field at the muon site

To unify the description of the possible magnetic structures in the tetragonal phase of $Ba_{1-x}K_xFe_2As_2$ (BKFA) we used the space group P4/mbm N127 that is the subgroup of index 4 of the parent group I4/mmm N139. This choice is dictated by the expected four-fold increase of the magnetic unit cell as compared to the parent I4/mmm primitive cell that is caused by the lowering of the translation symmetry. The P4/mbm subgroup has the same origin as the parent group I4/mmm and the basis (**a, b, c**) that is rotated by 45° in the *ab*-plane as compared to the I4/mmm basis (**a', b', c'**) with a=b=2a' and c=c'. In the P4/mbm setting the eight Fe atoms in the unit cell are in the – 8k (x, x+1/2, z) position. The 2e position of the As atoms and of the muon site in the I4/mmm notation are divided in the P4/mbm setting into the 4e – (0,0,$z_1$(As/μ)) and 4f - (0,1/2, $z_2$(As/μ)) positions. Respectively, the 4j position of the third muon site in the I4/mmm notation are divided in the P4/mbm setting into the 8j – (x, y, 1/2) and two 4g - (x, x+1/2, 0) positions. The primitive cell of BKFA in the P4/mbm setting is shown in Fig. S1.

The symmetry consideration of the possible ***2k***- and ***1k***- (or double-**Q** and single-**Q**) magnetic structures is based on the so called representation analysis of the magnetic degrees of freedom that are real and located on the magnetic ions and that are virtually assigned on the muon stopping sites [S5, S6]. The magnetic degrees of freedom, for a set of atoms at a given Wyckoff position, form a magnetic representation which is reducible and can be decomposed into irreducible representations (IR). The possible magnetic structures can be presented in terms of a linear combination of magnetic moments, ***L***, which transform under the symmetry operations as basic functions of a given IR. This is in accordance with the Landau concept that only one IR is realized at a phase transition for which ***L*** is a nonzero order parameter in the low symmetry phase.

Purely based on symmetry arguments one can make the following strict predictions for the local magnetic field that is seen in a zero-field μSR experiment. The complex magnetic structure does not give rise to a finite magnetic field at the muon site if the IR of its order parameter does not enter into the decomposition of the magnetic representation for the muon site.

This circumstance is illustrated below for the possible magnetic structures in the tetragonal phase of BKFA. For the following analysis it is important to note that the lowering of the translation symmetry in the ***2k***-structures is already accounted for by using a four times enlarged primitive unit cell. In the P4/mbm setting thus we can perform the symmetry

treatment for the Fe- and muon-site magnetic representations for the propagation vector $K_0$=(0, 0, 0).

To represent the order parameters of the respective ***2k***-magnetic structures, which can arise in the I4/mmm setting with the propagation vectors $\mathbf{k}_1$=(1/2, 1/2, 0) and $\mathbf{k}_2$=(-1/2, 1/2, 0), we introduce the following linear combinations ***L*** of the magnetic iron moments in the P4/mbm setting with $K_0$=(0, 0, 0).

$$\begin{aligned} \vec{F}^{(\pm)} &= 1/8[(\vec{m}_1+\vec{m}_2+\vec{m}_3+\vec{m}_4)\pm(\vec{m}_5+\vec{m}_6+\vec{m}_7+\vec{m}_8)]; \\ \vec{L}_1^{(\pm)} &= 1/8[(\vec{m}_1+\vec{m}_2-\vec{m}_3-\vec{m}_4)\pm(\vec{m}_5+\vec{m}_6-\vec{m}_7-\vec{m}_8)]; \\ \vec{L}_2^{(\pm)} &= 1/8[(\vec{m}_1-\vec{m}_2+\vec{m}_3-\vec{m}_4)\pm(\vec{m}_5-\vec{m}_6+\vec{m}_7-\vec{m}_8)]; \\ \vec{L}_3^{(\pm)} &= 1/8[(\vec{m}_1-\vec{m}_2-\vec{m}_3+\vec{m}_4)\pm(\vec{m}_5-\vec{m}_6-\vec{m}_7+\vec{m}_8)]. \end{aligned} \qquad (1)$$

The magnetic order parameters ***L*** consist of the Fourier components of the magnetic propagation vector, $\boldsymbol{K_o}$, in terms of the sub-lattice magnetic moments $m_\alpha$ with $\alpha$=1÷8. Similarly one can introduce linear combinations of the $\boldsymbol{K_0}$ - Fourier components of the magnetic fields $B_\alpha^{I,II}$ ($\alpha$=1÷4) at the muon positions with *4e* and *4f* site symmetry that are enumerated by I and II respectively. The respective staggered magnetic fields at these muon sites have the form:

$$\begin{aligned} \vec{F}^{(I,II)} &= \frac{1}{4}\left(\vec{B}_1^{(I,II)}+\vec{B}_2^{(I,II)}+\vec{B}_3^{(I,II)}+\vec{B}_4^{(I,II)}\right); \\ L_1^{(I,II)} &= \frac{1}{4}\left(\vec{B}_1^{(I,II)}+\vec{B}_2^{(I,II)}-\vec{B}_3^{(I,II)}-\vec{B}_4^{(I,II)}\right); \\ L_2^{(I,II)} &= \frac{1}{4}\left(\vec{B}_1^{(I,II)}-\vec{B}_2^{(I,II)}+\vec{B}_3^{(I,II)}-\vec{B}_4^{(I,II)}\right); \\ L_3^{(I,II)} &= \frac{1}{4}\left(\vec{B}_1^{(I,II)}-\vec{B}_2^{(I,II)}-\vec{B}_3^{(I,II)}+\vec{B}_4^{(I,II)}\right); \end{aligned} \qquad (2)$$

The quantities defined in Eqs. (1) and (2) can serve as the basic functions of the irreducible representations of the P4/mbm group with propagation vector $\boldsymbol{K_0}$=(0, 0, 0). The attribution of these basic functions to the IR of the tetragonal group I4/mbm is as shown in Table 1.

The following examples illustrate how to read the data of Table I. The magnetic structures which can be realized with the iron order parameters of a given IR give rise to staggered fields at the muon sites that transform by the same IR. For example, the magnetic structure which transforms according to the IR $\tau_5$ - $B_{1g}$ consists of the two order parameters $L_{3x}^{(-)}$-$L_{1x}^{(-)}$ and $L_{2z}^{(+)}$. According to Table I, both order parameter $L_{3x}^{(-)}$-$L_{1x}^{(-)}$ and $L_{2z}^{(+)}$ do not create finite dipolar fields at the (4e) muon stopping sites. At the same time, at the (4f) muon stopping sites they both create dipolar fields that are directed along the c-axis and have the same

| P4/mbm | $K_0=(0;\ 0;\ 0)$ | | | | |
|---|---|---|---|---|---|
| IR | **Fe** order parameters | Fields at muon sites (4e)-I | Frequency at $1\mu_B/Fe$ in MHz | Fields at muon sites (4f)- II | Frequency at $1\mu_B/Fe$ in MHz |
| $\tau_1-A_{1g}$ | $L_{3x}^{(-)}+L_{1y}^{(-)}$ | $L_{2z}^{(I)}$ | 52.84 | -- | 0 |
| $\tau_2-A_{1u}$ | $L_{1x}^{(+)}-L_{3y}^{(+)};\ F_z^{(-)}$ | $L_{3z}^{(I)}$ | 0 | $L_{3z}^{(II)}$ | 0 |
| $\tau_3-A_{2g}$ | $L_{1x}^{(-)}-L_{3y}^{(-)};\ F_z^{(+)}$ | $F_z^{(I)}$ | 0 | $F_z^{(II)}$ | 0 |
| $\tau_4-A_{2u}$ | $L_{3x}^{(+)}+L_{1y}^{(+)}$ | $L_{1z}^{(I)}$ | 52.03 | -- | 0 |
| $\tau_5-B_{1g}$ | $L_{3x}^{(-)}-L_{1y}^{(-)};\ L_{2z}^{(+)}$ | -- | 0 | $L_{2z}^{(II)}$ | 52.84 |
| $\tau_6-B_{1u}$ | $L_{1x}^{(+)}+L_{3y}^{(+)}$ | -- | 0 | -- | 0 |
| $\tau_7-B_{2g}$ | $L_{1x}^{(-)}+L_{3y}^{(-)}$ | -- | 0 | -- | 0 |
| $\tau_8-B_{2u}$ | $L_{3x}^{(+)}-L_{1y}^{(+)};\ L_{2z}^{(-)}$ | -- | 0 | $L_{1z}^{(II)}$ | 52.03 |
| $\tau_9-E_g$ | $\left\{\begin{matrix}F_x^{(+)}\\ -F_y^{(+)}\end{matrix}\right.;$ $\left\{\begin{matrix}L_{2y}^{(+)}\\ -L_{2x}^{(+)}\end{matrix}\right.;\ \left\{\begin{matrix}L_{1z}^{(-)}\\ L_{3z}^{(-)}\end{matrix}\right.$ | $\left\{\begin{matrix}F_x^{(I)}\\ -F_y^{(I)}\end{matrix}\right.;$ $\left\{\begin{matrix}L_{2y}^{(I)}\\ L_{2x}^{(I)}\end{matrix}\right.;$ | | $\left\{\begin{matrix}F_x^{(II)}\\ -F_y^{(II)}\end{matrix}\right.;$ $\left\{\begin{matrix}L_{2y}^{(II)}\\ -L_{2x}^{(II)}\end{matrix}\right.;$ | |
| $\tau_{10}-E_u$ | $\left\{\begin{matrix}L_{2x}^{(-)}\\ L_{2y}^{(-)}\end{matrix}\right.;$ $\left\{\begin{matrix}F_y^{(-)}\\ F_x^{(-)}\end{matrix}\right.;\ \left\{\begin{matrix}L_{3z}^{(+)}\\ -L_{1z}^{(+)}\end{matrix}\right.$ | $\left\{\begin{matrix}L_{1x}^{(I)}\\ -L_{1y}^{(I)}\end{matrix}\right.;$ $\left\{\begin{matrix}L_{3y}^{(I)}\\ L_{3x}^{(I)}\end{matrix}\right.;$ | | $\left\{\begin{matrix}L_{1x}^{(II)}\\ L_{1y}^{(II)}\end{matrix}\right.;$ $\left\{\begin{matrix}L_{3y}^{(II)}\\ L_{3x}^{(II)}\end{matrix}\right.;$ | |

***Table 1**: Symmetry of the order parameters of the possible Fe-based magnetic phases and the symmetry and magnitude of the respective staggered magnetic fields from Eq. (2) at the muon sites in the tetragonal phase of $Ba_{1-x}K_xFe_2As_2$ in P4/mbm setting for the magnetic propagation vector $\mathbf{K_0}$=(0, 0, 0).*

staggered structure $L_{2z}^{(II)}$. This is a strict result if we take the iron coordinates in the form Fe – 8k (x, x+1/2, z). However, there is the starting symmetry I4/mmm which we can reproduce by taking the iron coordinates as x=1/4, z=1/4 so that we get 8k (1/4, 3/4, 1/4). This additional, internal symmetry leads to the disappearance of the magnetic fields at some of the muon stopping sites.

The magnetic structures (order parameters), which do not give rise to a finite magnetic field at the muon site for x=1/4, z=1/4, are marked in "yellow". The "pink" color denotes the magnetic structures (order parameters) that cannot be detected by μSR for the given (4e) and (4f) muon stopping sites, even for an arbitrary choice of the x-and z-coordinates in Fe – 8k (x, x+1/2, z). All of these structures are illustrated in Fig. S2.

Note that structures marked in “yellow” can give rise to small, finite fields at the muon sites in the case of small, static deviations of the iron coordinates from the values x=1/4 and z=1/4. In this case the local fields and the resulting μSR precession frequencies will be more or less proportional to the amplitude of the deviations.

Below we summarize the outcome of the dipole field calculations for the magnetic order parameters with AF order along the c-axis for the case Fe – 8k (1/4, 3/4, 1/4). The magnetic fields are given in units of *MHz*, corresponding to the μSR precession frequency, $\nu_\mu = \frac{\gamma_\mu}{2\pi} \cdot B_\mu$ and the magnetic order parameters (linear combinations from Eq. (1)) in units of $\mu_B$.

The fields at the (4e) –muon sites with coordinates (0.0, 0.0, 0.1880) are:

$$\begin{pmatrix} B_x \\ B_y \\ B_z \end{pmatrix} = \begin{pmatrix} 28.52 & 0 & 0 \\ 0 & 28.52 & 0 \\ 0 & 0 & -57.04 \end{pmatrix} \begin{pmatrix} F_x^{(-)} \\ F_y^{(-)} \\ F_z^{(-)} \end{pmatrix} + \begin{pmatrix} 0 & 0 & 0 \\ 0 & 0 & 37.36 \\ 0 & 37.36 & 0 \end{pmatrix} \begin{pmatrix} L_{1x}^{(-)} \\ L_{1y}^{(-)} \\ L_{1z}^{(-)} \end{pmatrix} + \tag{3}$$

$$+ \begin{pmatrix} 0 & 59.96 & 0 \\ 59.96 & 0 & 0 \\ 0 & 0 & 0 \end{pmatrix} \begin{pmatrix} L_{2x}^{(-)} \\ L_{2y}^{(-)} \\ L_{2z}^{(-)} \end{pmatrix} + \begin{pmatrix} 0 & 0 & 37.36 \\ 0 & 0 & 0 \\ 37.36 & 0 & 0 \end{pmatrix} \begin{pmatrix} L_{3x}^{(-)} \\ L_{3y}^{(-)} \\ L_{3z}^{(-)} \end{pmatrix} +$$

The fields at the (4f) –muon sites with coordinates (0.5, 0.0, 0.312) are:

$$\begin{pmatrix} B_x \\ B_y \\ B_z \end{pmatrix} = \begin{pmatrix} \text{-28.52} & 0 & 0 \\ 0 & \text{-28.52} & 0 \\ 0 & 0 & 57.04 \end{pmatrix} \begin{pmatrix} F_x^{(-)} \\ F_y^{(-)} \\ F_z^{(-)} \end{pmatrix} + \begin{pmatrix} 0 & 0 & 0 \\ 0 & 0 & \text{-37.36} \\ 0 & \text{-37.36} & 0 \end{pmatrix} \begin{pmatrix} L_{1x}^{(-)} \\ L_{1y}^{(-)} \\ L_{1z}^{(-)} \end{pmatrix} + \tag{4}$$

$$+ \begin{pmatrix} 0 & 59.96 & 0 \\ 59.96 & 0 & 0 \\ 0 & 0 & 0 \end{pmatrix} \begin{pmatrix} L_{2x}^{(-)} \\ L_{2y}^{(-)} \\ L_{2z}^{(-)} \end{pmatrix} + \begin{pmatrix} 0 & 0 & 37.36 \\ 0 & 0 & 0 \\ 37.36 & 0 & 0 \end{pmatrix} \begin{pmatrix} L_{3x}^{(-)} \\ L_{3y}^{(-)} \\ L_{3z}^{(-)} \end{pmatrix} +$$

In the following Figure S2 we show the magnetic structures which do not give rise to a magnetic field at the muon site and thus to a finite μSR precession frequency. These structures are therefore not compatible with our experimental data in the t-AF state.

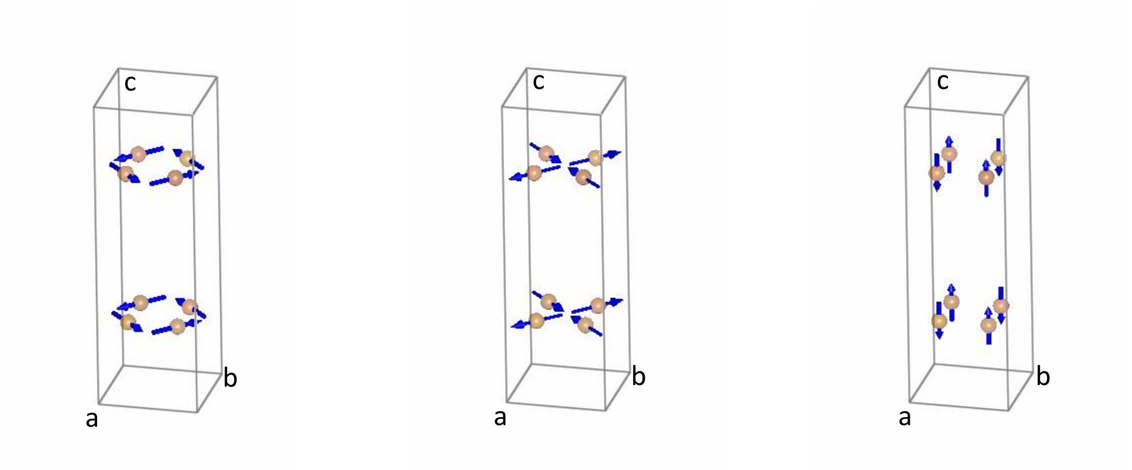


a) IR $\tau_2$ $L_{1x}^{(+)} - L_{3y}^{(+)};$ b) IR $\tau_6$ $L_{1x}^{(+)} + L_{3y}^{(+)}$ c) IR $\tau_5$ $L_{2z}^{(+)}$

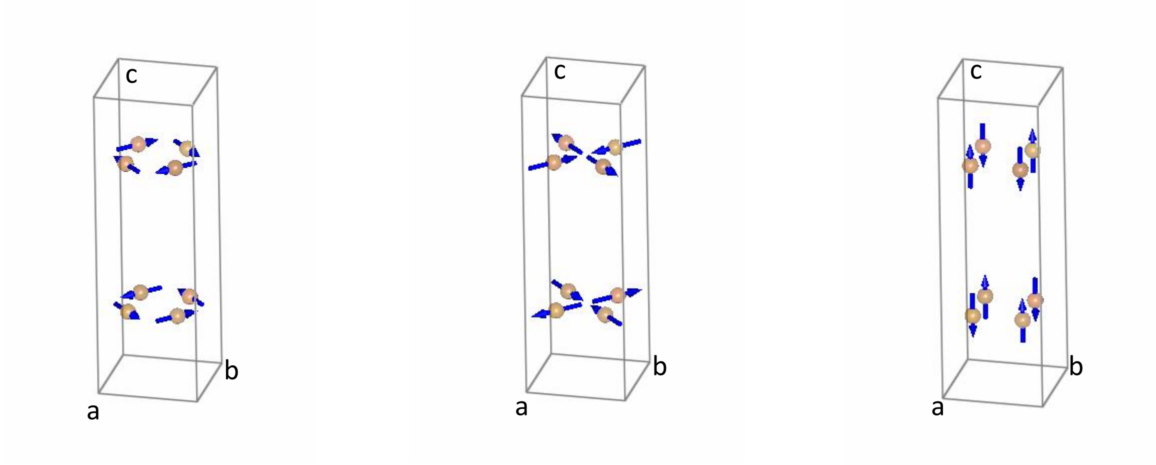


d) IR $\tau_3$ $L_{1x}^{(-)} - L_{3y}^{(-)};$ e) IR $\tau_7$ $L_{1x}^{(-)} + L_{3y}^{(-)}$ f) IR $\tau_8$ $L_{2z}^{(-)}$

***Figure S2:*** *Double-Q magnetic structures in P4/mbm setting which preserve the C4 symmetry and do not create a magnetic dipole field at the muon sites. Only the iron atoms are shown. The structures in* ***a); b);*** *and* ***c)*** *exhibit a FM order along the c-axis, the ones in* ***d); e); f)*** *a corresponding AFM order.*

In Figure S3 we show the non-collinear double-Q structures with in-plane oriented magnetic moments which create a finite dipolar magnetic field at the muons sites of tetragonal BKFA. The indicated μSR precession frequencies have been obtained using Eqs (2) and (3) under the assumption that each Fe ion has a magnetic moment of 1 $\mu_B$. These are much larger than the experimental ones and also than the calculated ones for the single-Q magnetic order (see below and Fig. S6) in the o-AF state and can therefore also be excluded as candidates for the t-AF state.

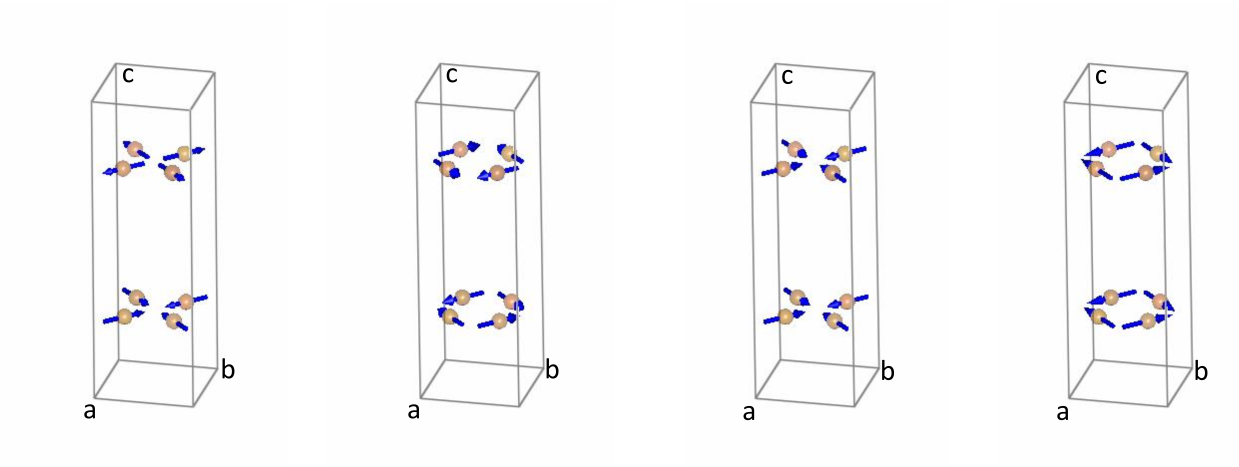


52.84 MHz at 1$\mu_B$/Fe

52.03 MHz at 1$\mu_B$/Fe

a) IR $\tau_1$ $L_{3x}^{(-)}+L_{1y}^{(-)}$; b) IR $\tau_5$ $L_{3x}^{(-)}-L_{1y}^{(-)}$ c) IR $\tau_4$ $L_{3x}^{(+)}+L_{1y}^{(+)}$; d) IR $\tau_8$ $L_{3x}^{(+)}-L_{1y}^{(+)}$

***Figure S3****: Non-collinear double-Q structures with in-plane oriented moments in the tetragonal phase which create a finite magnetic dipole field at the muons sites. Shown are only the iron atoms. Panels* ***a)*** *and* ***b)*** *show the structures with AFM order along the c-axis, panels* ***c)*** *and* ***d)*** *the corresponding structures with FM order. The indicated μSR precession frequencies are calculated using Eqs. (3) and (4). They are very similar and thus are likely within the error bar of a typical μSR experiment.*

For the double-Q magnetic structures shown above, each Fe ion has the same magnetic moment which is assumed to amount to 1 $\mu_B$. However, there exists also the possibility of a so-called inhomogeneous double-Q magnetic structure for which the magnetic moment becomes zero for half of the Fe sites. It is described by the PC42/ncm magnetic group symmetry and preserves the C4 symmetry. In our P4/mbm setting this structure corresponds to the linear combination $\boldsymbol{L_{1z}^{(-)}+L_{3z}^{(-)}}$**.** In the I4/mmm setting, it is described by the linear combination of the order parameter $\eta_z(k1)+\eta_z(k2)$ which belong to different arms of the K13-star. This structure is shown below in Fig. S4. The calculations show that it yields a moderate µSR precession frequency that is lower than the one in the orthorhombic phase (see below and Fig. S6 in agreement with the experimental data. In contrast to other magnetic phases, the coexistence of the nonmagnetic (S=0) and magnetic (S≠0) sites may indicate an alteration of the iron spin states of the neighboring ions. A large variation of the iron spin state is indeed not uncommon to the parent compounds of the iron superconductors for which the magnetic moment varies from the high spin state with S=2 and a moment of 3.5$\mu_B$/Fe in $Rb_2Fe_4Se_5$ to the low spin state with S=0 in FeSe.

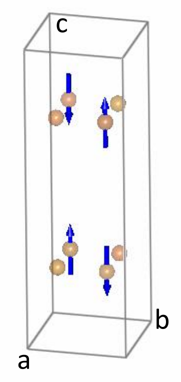


µSR frequency of 26.4 MHz at 1$\mu_B$/Fe .

***Figure S4***: *Inhomogeneous, double-Q magnetic structure, $L_{1z}^{(-)}+L_{3z}^{(-)}$, with alternating zero and nonzero magnetic moment at the iron sites with $P_c4_2/ncm$ magnetic group symmetry according to Ref. [S8]. The indicated µSR precession frequency has been calculated using Eqs. (3) and (4). Shown are only the iron atoms. This is the double-Q magnetic structure that is compatible with our µSR data.*

Next, we consider the somewhat artificial case of an AFM structure with different but nonzero magnetic moments on the two iron sub-lattices as is shown on Fig. S7. Such a magnetic structure, for example with alternating magnetic moments of 1 $\mu_B$/Fe and 0.7 $\mu_B$/Fe can reproduce the experimentally observed change of the μSR precession frequency at orthorhombic-tetragonal transition by about 14%. Nevertheless, it does not preserve the $C_4$ symmetry and thus should lead to a detectable orthorhombic distortion that has not been observed in the x-ray experiments (see Fig. 1 of the paper).

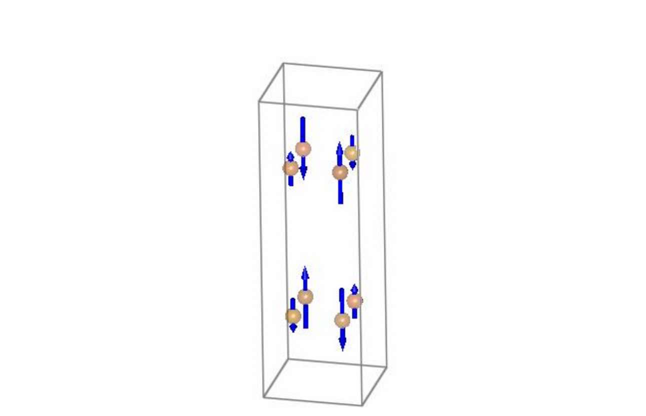

μSR frequency of 32.33 MHz at $M_1$=1$\mu_B$/Fe and $M_{12}$=0.7$\mu_B$/Fe.

***Figure S5:*** *Magnetic structure with alternating but finite magnetic moments on the Fe sites that is analogous to the one shown in Fig. S4 but does not preserve $C_4$ axis and thus should give rise to a detectable orthorhombic distortion.*

Finally we discuss the so-called single-Q magnetic structures which require an orthorhombic structure since they break the C4 symmetry. From the magnetic symmetry point of view the symmetry reduction that takes place at the transition from the paramagnetic tetragonal I4/mmm1' phase to the magnetic orthorhombic CAmca (or FCmm'm') phase can be ascribed as a condensation of the magnetic order parameter $\eta_{xy}(k_1)$ or $\eta_{\bar{x}y}(k_1)$ in the I4/mmm setting. Here two order parameters with different translation symmetry form two different orthorhombic domains. In our P4/mbm setting for the paramagnetic phase these two domains of the orthorhombic magnetic phase can be described as a condensation of the $L_{3x}^{(-)}$ and $L_{1y}^{(-)}$ order parameters, respectively. The structure with the out-of-plane direction of the magnetic moments in the tetragonal AF phase can be obtained by a continuous rotation of the magnetic moments in the ac-plane. The respective magnetic structures are shown in Fig. S6. Note that

in accordance with Eqs. (2-3) all of them give rise to the same μSR precession frequency which for a Fe moment of 1 $\mu_B$ amounts to 32.3 MHz.

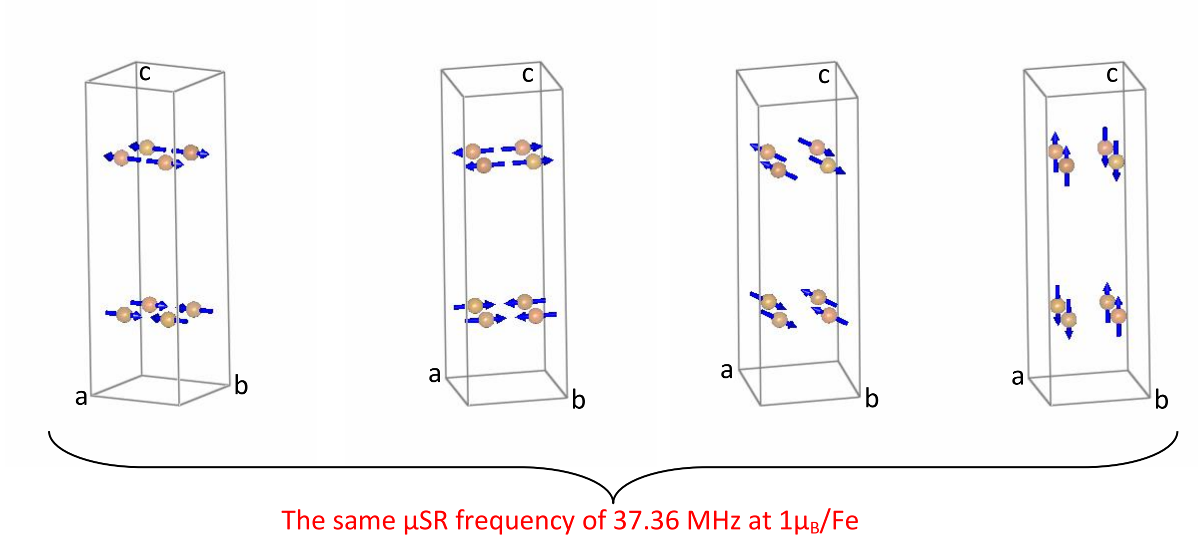


a) $L_{1y}^{(-)}$ ; b) $L_{3x}^{(-)}$ - $C_A mca$; c) $\sin\alpha L_{3x}^{(-)} + \cos\alpha L_{3z}^{(-)}$ ; d) $L_{3z}^{(-)}$ -$P_C ccn$ or $C_A 222_1$

***Figure S6:*** *Magnetic structures and their order parameters in the orthorhombic state. All phases preserve the same pattern (type) of the exchange interactions.* ***a)*** *and* ***b)*** *show the two domain state of the stripe-like AF order that is realized in the orthorhombic phase;* ***c)*** *a spin rotated phase with an arbitrary rotation angle α.* ***d)*** *the pure out-of-plane magnetic order that has been suggested in Ref. [S9] as the magnetic structure in the tetragonal AF phase. This structure breaks the $C_4$ symmetry of the tetragonal crystal structure. Note that the μSR precession frequencies remain the same in accordance with Eqs. (3) and (4), under the continuous rotation from the pure in-plane to the pure out –of-plane structure.*

At last we mention the μSR precession frequency at the third muon site for the relevant magnetic structures under the assumption of a magnetic moment of 1 $\mu_B$/Fe. In the o-AF state (for the structure shown in Fig. S6(b)) it amount to about 8.9 MHz; whereas in the t-AF state (for the structure shown in Fig. S4) it is reduced to about 6.5 MHz. Moreover, the direction of the field at this third muon site is parallel to the c-axis in the o-AF state and parallel to the ab-plane in the t-phase, similar to local magnetic field at the main muon site.

## Orientation of the local field from ZF-μSR

The $c$-axis orientation of $\vec{B}_\mu$ in the o-AF state and its in-plane orientation in the t-AF state are also seen from the ZF-μSR data. Figure S7(a) shows the ZF-μSR curves as obtained with the so-called forward and backward counters that are probing the asymmetry of the positron emission rate along the c-axis direction of the BKFA crystal (which is parallel to the $z$-axis in Fig. S7(b)). These counters probe the evolution of the $c$-axis component of the muon spin polarization.

For the curve at 35 K in the o-AF state it is evident that the amplitude of the oscillating signal is essentially zero. This is an unambiguous proof that the precession axis of $\vec{S}_\mu$ and thus the direction of $\vec{B}_\mu$ is parallel to the $c$-axis of the BKFA crystal.

To the contrary, for the curve at 20K in the t-AF state the amplitude of the precessing signal is rather large. This is consistent with the in-plane orientation of $\vec{B}_\mu$ which has been inferred from the TF-μSR data as shown in Fig. 4 of the paper.

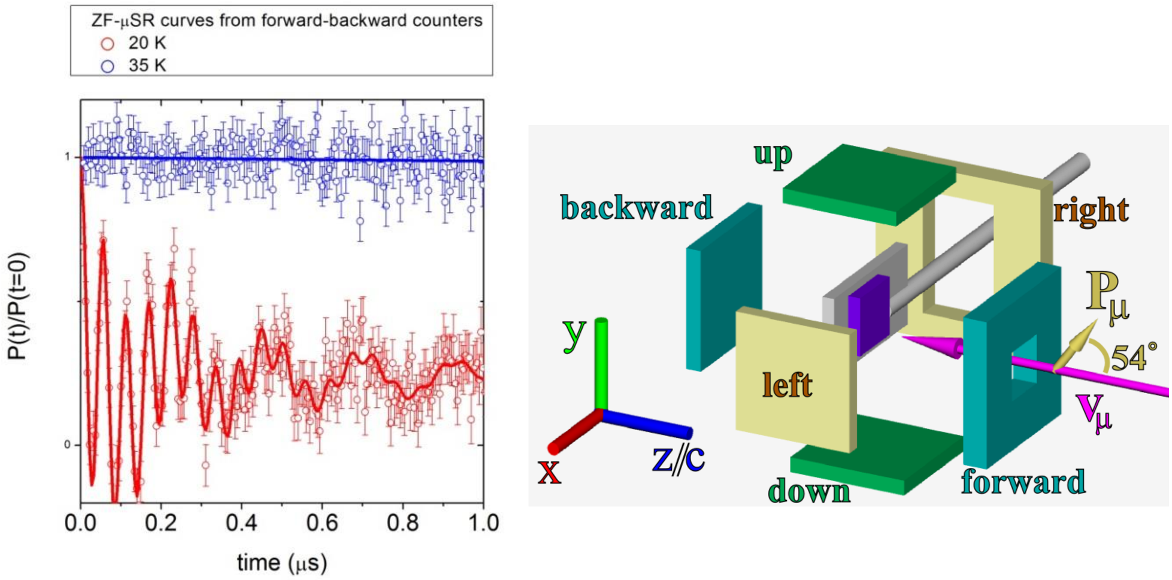


***Figure S7:*** *(a) ZF-μSR spectra as obtained with the forward and backward positron counters for which the symmetry axis is parallel to the c-axis of the BKFA crystal. The absence of a precessing signal at 35 K confirms the c-axis orientation of* $\vec{\boldsymbol{B}}_{\boldsymbol{\mu}}$ *in the o-AF state. Likewise, the large amplitude of the precessing signal at 20K is consistent with the in-plane orientation of* $\vec{\boldsymbol{B}}_{\boldsymbol{\mu}}$ *in the t-AF state .(b) A sketch showing the experimental geometry and the three detector*

*sets. The sample, shown in dark blue, has its c-axis aligned with the z-axis and the incoming muon beam.*

## Analysis of the x-ray data

In the o-AF state below $T^{N1} \approx 72K$ we observe with x-ray diffraction the tetragonal (1,1,14) Bragg-peak split into two peaks, as expected, showing a tetragonal to orthorhombic structural transition. Below we denote the distance in reciprocal space in the (1,1,0) direction as $Q_{x'}$ for which the corresponding direction in real space is along the nearest neighbor Fe-Fe bond. The splitting of the Bragg peak in the $Q_{x'}$ direction is shown in Fig. 1(a) and (c) of the main paper and in Fig. S8(c). In the t-AF phase between $T^{N2}$ and $T^{N3}$, the intensity of these split orthorhombic peaks decreases strongly whilst a third Bragg-peak at intermediate $Q_{x'}$ grows in intensity. This is shown in Fig. S8(a) which plots the diffracted x-ray intensity in a region of reciprocal space around the (1,1,14) Bragg-peak in the t-AF phase at T=21 K. The main feature is this Bragg-peak at intermediate $Q_{x'}$ = 0.3631 Å$^{-1}$ whilst only a weak remnant of one of the split orthorhombic peaks can be seen at larger $Q_{x'}$ demonstrating that the majority of the sample is tetragonal in the t-AF phase. As shown in Fig. 1(c) of the main paper, below $T^{N3}$ we observe again diffractograms essentially the same, but with smaller lattice parameters, as those for the higher temperature o-AF phase between $T^{N1}$ and $T^{N2}$.

In order to estimate what fraction of the sample remains with this orthorhombic symmetry in the t-AF phase, each of the three Bragg peaks were fitted to an asymmetric 2-dimensional Gaussian function;

$$I = A \exp\left[-\frac{(Q_{x'} - \mu_{x'})^2}{2\sigma_{x'}^2} - \frac{(Q_z - \mu_z)^2}{2\sigma_z^2}\right]$$

The volume of this function is $2\pi A\sigma_{x'}\sigma_z$ which we call here the weight. The weight of the t-AF peak and combined weight of the t-AF peaks are plotted as a function of temperature in Fig. 1(d) of the main paper. The fitted center of each peak, $\mu_{x'}$, is plotted in Fig.1(c).

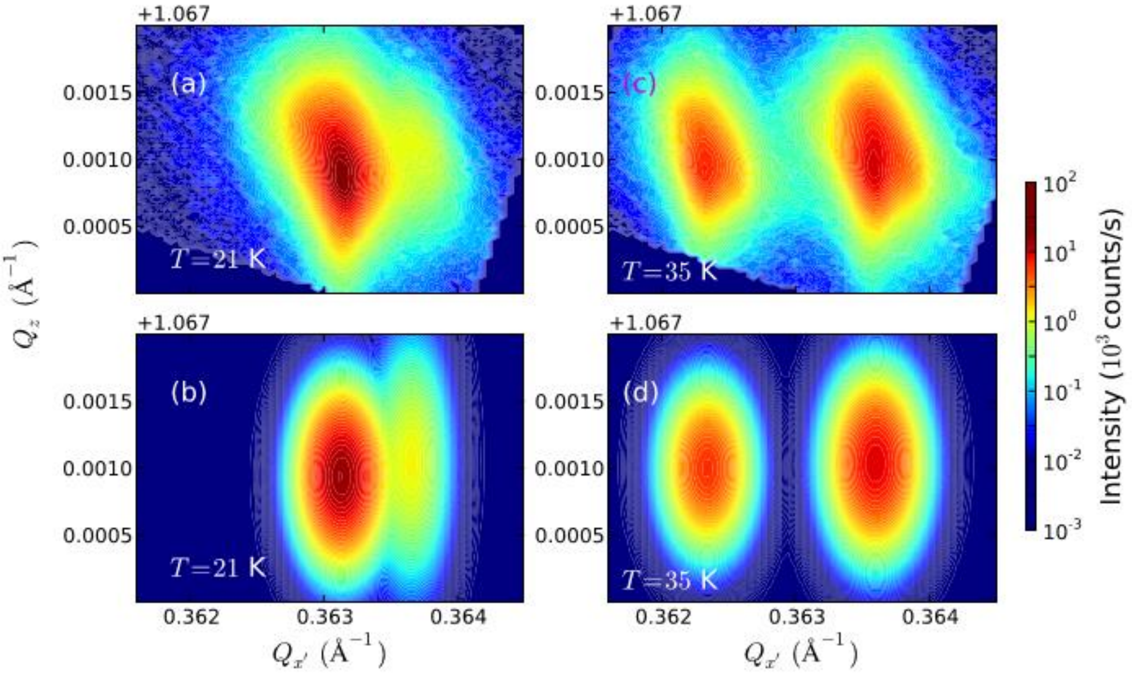


***Figure S8:*** *(a) X-ray diffractometry data at T=21 K (in the t-AF phase) in a region of reciprocal space around the (1,1,14) Bragg peak. Note the log scale. Panel (b) shows a fit to the T=21 K data. Panels (c) and (d) show the data and fit at T=35K (in the o-AF phase), respectively.*

The full-width-at-half-maximum of the peaks in $Q_{x'}$ is ~$3.5\text{x}10^{-4}$ $Å^{-1}$ for both the o-AF and t-AF phases, four times larger than our experimental resolution, which already shows any orthorhombic splitting of the (1,1,14) Bragg peak in the t-AF state is small. An estimate of the upper limit of the orthorhombic splitting of the (1,1,14) Bragg peak in the t-AF state can be obtained by assuming that the peak is composed of two overlapping peaks. We fix the amplitude of these two putative peaks at half the total amplitude of the fitted single peak, $A_1$=$A_2$=A/2, and then fit the data by freely varying the other variables. The fitted centers of these two peaks, $\mu_{x1}$, $\mu_{x2}$, differ by ~$5\text{x}10^{-5}$ $Å^{-1}$. This splitting is two orders of magnitude smaller than the splitting in the o-AF state where $\mu_{x1}$-$\mu_{x2}$=$1.2\text{x}10^{-3}$ $Å^{-1}$.

## References

[S1] I. M. Reznik, F. G. Vagizov, and R. Troc, Phys. Rev. B **51**, 3013 (1995)RS1.

[S2] See http://elk.sourceforge.net.

[S3] J. P. Perdew and Yue Wang, Phys. Rev. B 45, 13244 (1992).

[S4] J. P. Perdew, A. Ruzsinszky, G. I. Csonka, O. A. Vydrov, G. E. Scuseria, L. A. Constantin, X. Zhou, and K. Burke, Phys. Rev. Lett. 100, 136406 (2008)

[S5] E. F. Bertaut, Acta Crystallogr., A **24**, 217 (1968); J. Phys. (France) **32**, 462 (1971); J. Magn. Magn. Mater. **24**, 267 (1981).

[S6] W. Opechowski, T. Dreyfus, Acta Crystallogr. A **27**, 470 (1971)

[S7] Y. A. Izyumov, V. E. Naish, and R. P. Ozerov, *Neutron Diffraction of Magnetic Materials* Consultants Bureau, Plenum Publishing Corporation, New York, 1991.

[S8] D. D. Khalyavin, S. W. Lovesey, P. Manuel, F. Krüger, S. Rosenkranz, J. M. Allred, O. Chmaissem, and R. Osborn, Phys. Rev. B **90**, 174511 (2014)

[S9] F. Waßer, A. Schneidewind, Y. Sidis, S. Wurmehl, S. Aswartham, B. Büchner and M. Braden, Phys. Rev. B **91**, 060505 (2015).
